# Supplementary material for: How Transformers Utilize Multi-Head Attention in In-Context Learning? A Case Study on Sparse Linear Regression
Source: arXiv:2408.04532 source file (2024-08-08)
Supplement: Supplementary file 4 [file proof_iso.tex]

\section{Proof for Theorem~\ref{thm:identitycase}}\label{sec:identitycase}
To simplify the notation, we use $\hat{\wb}_t$ to denote $\twgd^t$ and $\wb_t$ to denote $\wgd^t$. 
\subsection{Proof for the upper bound of the excess risk}

When $\Sigmab=\Ib$, by \Eqref{eq: our_algo_decom}, we have
\begin{align*}
\cE\paren{\wpre_t}=
\underbrace{\normm{\Rh{{\paren{\Ib-\eta\Sigmah}^t}\Rl\ws}}_2^2}_{\mathrm{Bias}}
    +\underbrace{\eta^2\normm{\Rh\paren{\frac{1}{n}{\sum_{i=1}^{t}\paren{\Ib-\eta\Sigmah}^{i-1}}\Xt^\top\epsb}}_2^2}_{\mathrm{Variance}}.
\end{align*}
Following the proof of Theorem~\ref{thm: main}, it holds that
\begin{align*}
     \mathrm{Variance}\lesssim
    \eta t \log t\cdot{\frac{\sigma^2\log\paren{d/\delta}}{n}+\frac{\sigma^2sd\log^2\paren{d/\delta}}{n^2}}
\end{align*}
\whp, when $n\gtrsim {t^2sd^{2/3}}$

Similar to the proof of Lemma~\ref{lem: c.2}, we can prove that
\begin{align*}
    &\hat{r}_i\geq \frac{r_i}{2}~~\forall i\in \cS,
    &\hat{r}_i\lesssim 1~~\forall i,
\end{align*}
\whp.

When $\Sigmab=\Ib$, by Lemma~\ref{lem: concentration_covariance}, we have that 
\begin{align*}
    \normm{\Rh\Sigmah\Rh-\Rb\Sigmab\Rb}_2\lesssim \frac{\beta^2}{t}
\end{align*}
holds with probability at least $1-\delta$, when $n\gtrsim \frac{t^2\normm{\ws}_1^2d^{2/3}}{\beta^4}$. As a result, $\Rb\Sigmab\Rb-\frac{\beta^2}{t}\cdot \Ib\preceq \Rh\Sigmah\Rh$.
Hereafter, we condition on the above events. 
For the bias term, we have
\begin{align*}
    \normm{\Rh{{\paren{\Ib-\eta\Sigmah}^t}\Rl\ws}}_2^2&\leq \normm{\Rh}^2_2\cdot\normm{{{\paren{\Ib-\eta\Sigmah}^t}\Rl\ws}}_2^2\notag\\
    &\leq \ws^\top\Rl{\paren{\Ib-\eta\Sigmah}^{2t}}\Rl\ws\notag\\
    &\lesssim \ws^\top\Rl{\paren{\Ib-\eta\paren{\Rb\Sigmab\Rb-\frac{\beta^2}{t}\cdot\Ib}}^{2t}}\Rl\ws\notag\\
    &=\sum_{i\in \cS}\paren{w^\star_{i}/\hat{r}_{i}}^2\cdot \paren{1-\eta\paren{(w^\star_i)^2-\frac{\beta^2}{t}}}^{2t}\notag\\
    &\leq s\cdot \paren{1-\eta\beta^2/2}^{2t},
\end{align*}
where the last line is by the definition of $\beta$.
When $t\gtrsim \log\paren{\frac{\sigma^2}{ns}}/\paren{2\log\paren{1-\eta\beta^2/2}}$, we have
\begin{align}\label{eq: iso_bias}
     \mathrm{Bias}=\normm{\Rh{{\paren{\Ib-\eta\Sigmah}^t}\Rl\ws}}_2^2\leq \frac{\sigma^2}{n}.
\end{align}
When $\eta\beta^2/2\leq 1/2$, there exist a $c>0$, such that 
\begin{align*}
   \log\paren{1-\eta\beta^2/2}\geq c\eta\beta^2/2.
\end{align*}
Hence, the variance term is bounded by
\begin{align}\label{eq: iso_var}
    \mathrm{Variance}&\lesssim
    \eta t \log t\cdot\paren{\frac{\sigma^2\log\paren{d/\delta}}{n}+\frac{\sigma^2\normm{\ws}_1^2d\log^2\paren{d/\delta}}{n^2}}\notag\\
    &\lesssim \frac{\sigma^2{\log^2\paren{ns/\sigma^2}\log^2\paren{d/\delta}}}{\beta^2}\cdot\paren{\frac{s}{n}+\frac{ds}{n^2}},
    \end{align}
    where the last line is by $\normm{\ws}_1\leq s\cdot \normm{\ws}_2^2=s$ and $\eta t\lesssim \frac{\log\paren{ns/\sigma^2}}{\beta^2}$.
    Combining \Eqref{eq: iso_bias} and \Eqref{eq: iso_var}, we have that
    \begin{align*}
        \cE\paren{\wpre_t}\lesssim \frac{\sigma^2}{n}+\frac{\sigma^2{\log^2\paren{ns/\sigma^2}\log^2\paren{d/\delta}}}{\beta^2}\cdot\paren{\frac{1}{n}+\frac{ds}{n^2}}\lesssim \frac{\sigma^2{\log^2\paren{ns/\sigma^2}\log^2\paren{d/\delta}}}{\beta^2}\cdot\paren{\frac{1}{n}+\frac{ds}{n^2}},
    \end{align*}
    when $n\gtrsim \frac{t^2sd^{2/3}}{\beta^4}\geq \frac{t^2\normm{\ws}_1^2d^{2/3}}{\beta^4}$ and $t\gtrsim \frac{\log\paren{ns}}{\eta\beta^2}$.
    When $w^{\star}_i\in \mathsf{U}\{-1/\sqrt{s},1/\sqrt{s}\}$, $\beta=1/\sqrt{s}$. In this case, 
        we have that
    \begin{align*}
        \cE\paren{\wpre_t}\lesssim {\sigma^2{\log^2\paren{ns/\sigma^2}\log^2\paren{d/\delta}}}\cdot\paren{\frac{s}{n}+\frac{ds^2}{n^2}},
    \end{align*}
    when $n\gtrsim {t^2s^3d^{2/3}}$ and $t\gtrsim \frac{\log\paren{ns}}{\eta s}$.
