# Supplementary material for: How Transformers Utilize Multi-Head Attention in In-Context Learning? A Case Study on Sparse Linear Regression
Source: arXiv:2408.04532 source file (2024-08-08)
Supplement: Supplementary file 6 [file notation.tex]

% \section{Theoretical Analysis of the Preprocess-then-optimize Algorthm}\label{sec:notation}

% \subsection{Notations}
% For two functions $f(x) \geq 0$ and $g(x) \geq 0$ defined on the positive real numbers ($x > 0$), we write $f(x) \lesssim g(x)$ if there exists two constants $c,x_0 > 0$  such that $\forall x \geq x_0$, $f(x) \leq c \cdot g(x)$; we write $f(x) \gtrsim g(x)$ if $g(x) \lesssim f(x)$; we write $f(x) \backsimeq g(x)$ if $f(x) \lesssim g(x)$ and $g(x) \lesssim f(x)$. If $f(x) \lesssim g(x)$, we can write $f(x)$ as $O(g(x))$. We can also write write $f(x)$ as $\tilde{O}(g(x))$ if there exists a constant $k > 0$ such that $f(x) \lesssim g(x) \log^{k}(x)$.


% \subsection{Theoretical results}
% We first provide the upper bound of the excess risk for $\cE(\twgd^t)$ and $\cE(\wgd^t)$ respectively.
% \begin{theorem}\label{thm: main}
% Denote $\cS:=\{i:w^\star_i\neq 0\}$ and $\Rb=\mathsf{diag}\set{r_1,\ldots, r_d}$, where ${r_j}=\sum_{i=1}^d w^\star_i\Sigma_{ij}$. Suppose that there exist a $\beta>0$ such that $\min_{i\in\cS}\abs{r_i}\geq \beta$, $\normm{\Rb}_2,\normm{\Sigmab}_2, \normm{\ws}_2\simeq O\paren{1}$ and $n\gtrsim 1/\beta^2\cdot t^2s \cdot\big(\tr^{2/3}\paren{\Sigmab}+\tr\paren{\Rb\Sigmab\Rb}\big)\cdot\mathrm{poly}\paren{\log\paren{d/\delta}}$. Then set $\eta\lesssim 1/\normm{\Rb\Sigmab\Rb}_2$ and $
% \eta t\simeq \frac{1}{\beta}\cdot \big({\frac{\sigma^2\tr\paren{\Rb\Sigmab\Rb}\log\paren{d/\delta}}{n}+\frac{\sigma^2s\tr\paren{\Sigmab}\log^2\paren{d/\delta}}{n^2}}\big)^{-1/2}$, it holds that
% \begin{align*}
% \cE\paren{\twgd^t}
%     &\lesssim \frac{\log t}{\beta}\sqrt{{\frac{\sigma^2\tr\paren{\Rb\Sigmab\Rb}\log\paren{d/\delta}}{n}+\frac{\sigma^2s\tr\paren{\Sigmab}\log^2\paren{d/\delta}}{n^2}}},
% \end{align*}
% \whp.
% \end{theorem}
% Theorem \ref{thm: main} provides an upper bound on the excess risk achieved by the preprocess-then-optimize algorithm, where we tuned learning rate $\eta$ to balance the bias and variance error. Then, it can be seen that the risk bound is valid if $\tr\paren{\Rb\Sigmab\Rb}/n\rightarrow 0$ and $\tr(\bSigma) s/n^2\rightarrow 0$ when $n\rightarrow \infty$. This can be readily satisfied if we have $\|\wb^*\|_2$ and $\tr(\bSigma)$ be bounded by some reasonable quantities that are independent of the sample size $n$, which are the common assumptions made in many prior works \citep{zou2022risk,zou2021benefits,bartlett2020benign}. Besides, it can be also seen that the excess risk bound explicitly depends on the sparsity parameter $s$ and lower sparsity implies better performance. This implies the ability of the proposed preprocess-then-optimize for discovering and leveraging the nice sparse structure of the ground truth. 

% As a comparison, the following theorem states the excess risk bound for the standard gradient descents on the raw features. To make a fair comparison, we consider using the same number of steps but allow the step size to be tuned separately. 



% \begin{theorem}\label{thm:original_GD_general}
% Suppose that $\normm{\Sigmab}, \normm{\ws}_2\simeq O\paren{1}$ and $n\gtrsim t^2\paren{\tr\paren{\Sigmab}+\log\paren{1/\delta}}$. When $\eta\lesssim 1/\normm{\Sigmab}_2$ and $\eta t\simeq\paren{\frac{\sigma^2\tr\paren{\bSigma}\log\paren{d/\delta}}{n}}^{-1/2}$, it holds that  
% \begin{align*}
% \cE\paren{\wgd^t}\lesssim
%    \log t\cdot \sqrt{\frac{\sigma^2\tr\paren{\bSigma}\log\paren{d/\delta}}{n}},
% \end{align*}
% \whp.

% \end{theorem}
% We are now able to make a rough comparison between the excess risk bounds in Theorems \ref{thm: main} and \ref{thm:original_GD_general}. 
% Then, it is clear that $\cE(\twgd^t)\lesssim \cE(\wgd^t)$
% requires $\tr(\Rb\bSigma\Rb)/\beta^2\lesssim \tr(\bSigma)$ and $s/(n^2\beta^2)\le 1/n$. Specifically, we can consider the case that 
%  $\bSigma$ to be a diagonal matrix, assume $w^\star_i\sim \mathsf{U}\{-1/\sqrt{s}, 1/\sqrt{s}\}$ has a restricted uniform prior for $i\in\cS$ and $\min_{i\in\cS}\bSigma_{ii}\ge 1/\kappa$ for some constant $\kappa >1$, we can get  $\beta \ge \sqrt{1/(s\kappa^2)}$, thus $\tr(\Rb\bSigma\Rb)/\beta^2 \le \kappa^2\sum_{i:w^\star_i\neq 0}\bSigma_{ii}$ and $s/(n^2\beta^2)\le \kappa^2s^2/n^2$. Note that $|\cS|=s\ll d$, then if the covariance matrix $\bSigma$ has a flat eigenspectrum such that $\sum_{i\in\cS}\bSigma_{ii}\ll \sum_{i\in[d]}\bSigma_{ii}=\tr(\bSigma)$, we have $\tr(\Rb\bSigma\Rb)/\beta^2 \le \tr(\bSigma)$ and $s/(n^2\beta^2)\le \kappa^2s^2/n$ if $s=o\big(\min\{d,\sqrt{n}\}\big)$. This suggests that the preprocess-then-optimization algorithm can outperform the standard gradient descent for solving a sparse linear regression problem with $s=o\big(\min\{d,\sqrt{n}\}\big)$.



% To make a more rigorous comparison, we next consider the example where $x_i\iid \mathsf{N}\paren{\zerob,\Ib}$, based on which we can get the upper bound for our algorithm and the lower bound for OLS, ridge regression, and finite-step GD. 
% \begin{theorem}[Theorem \ref{thm:identitycase}, restated]\label{thm:identitycase_restate}
% Suppose $\cS$ with $\abs{\cS}=s$ is selected such that each element is chosen with equal probability from the set $\set{1,2,\ldots,d}$ and $w^\star_i\sim \mathsf{U}\{-1/\sqrt{s}, 1/\sqrt{s}\}$ has a restricted uniform prior for $i\in\cS$, $ \normm{\ws}_2\simeq \Theta\paren{1}$ and $n\gtrsim t^2s^3d^{2/3}$. Then there exists a choice of $\eta$ and $t$ such that
% \begin{align*}
% {\cE}\paren{\twgd^t}\lesssim 
%    \sigma^2{\log^2\paren{ns/\sigma^2}\log^2\paren{d/\delta}}\cdot\paren{\frac{s}{n}+\frac{ds^2}{n^2}},
% \end{align*}
% \whp. Besides, let $\wla$ be the ridge regression estimator with regularized parameter $\lambda$, and $\wols$ be the OLS estimator, it holds that
% \begin{align*}
% &\EE_{\ws}\brac{\cE\paren{\wb}}\gtrsim 
%     \begin{cases}
%         {\frac{\sigma^2d}{n}}&n\gtrsim d+\log\paren{1/\delta}\\
%        1-\frac{n}{d}+{\frac{\sigma^2n}{d}}&d\gtrsim n+\log\paren{1/\delta}, 
%     \end{cases}
% \end{align*}
% \whp, where $\wb\in\{\wla,\wols,\wgd^t\}$.
% \end{theorem}
% It can be seen that for a wide range of under-parameterized and over-parameterized cases, $\twgd^t$ has a smaller excess risk than ridge regression, standard gradient descent, and OLS. In particular, consider the setting $\sigma^2=1$, in the over-parameterized setting that $d\gtrsim n$, the excess risk bound of preprocess-then-optimize is $\tilde O(ds/n^2)$, which also outperforms the $\tilde \Omega(1)$ bound achieved by OLS, ridge regression, and standard gradient descent if the sparsity satisfies $s=O(n^2/d)$ (in fact, this condition can be certainly removed as ${\cE}(\twgd^t)$ also has a naive upper bound $\tilde O(1)$).  In the under-parameterized case that $d\lesssim n$, it can be readily verified that the data preprocessing can lead to a $\tilde O(s/n)$ excess risk, which is strictly better than the $\tilde \Omega(d/n)$ risk achieved by OLS, ridge regression, and standard gradient descent. Moreover, it is well known that Lasso can achieve $\tilde O(s/n)$ excess risk bound in the setting of Theorem \ref{thm:identitycase}. Then, by comparing with our results, we can also conclude that the proprocess-then-optimize algorithm can be comparable to Lasso up to logarithmic factors when $d\lesssim n$, while becomes worse when $d\gtrsim n$.
